# Supplementary material for: Consistency Training with Virtual Adversarial Discrete Perturbation
Source: arXiv:2104.07284 source file (2022-04-28)
Supplement: Supplementary file 1 [file 14_experimental_details_appendix.tex]

Our implementation is based on huggingface\footnote{\url{https://github.com/huggingface/transformers}}~\citep{wolf-etal-2020-transformers}.
In total, our method requires a single backward operation and a forward operation for generating the virtual adversarial samples, where each refinement step would additionally incur a single forward step. 
Our method takes approximately 2.5 times the standard training where the time complexity is similar or less than the recently introduced relevant methods~\citep{jiang2019smart, ng2020ssmba}.

During SSL experiments, we set the batch size to 8 for the labeled and 24 for the unlabeled data with the maximum sequence length of 256.
Also, we adopt some training tactics from UDA~\citep{xie2019unsupervised} during SSL to our method and the baselines, namely training signal annealing and sharpening, which moderately improves the performance.
The former is not to train overconfident samples, which is applied to the labeled data, and the latter is for sharpening the original samples' predictions for the unlabeled data.
However, we did not apply sharpening to the VAT baseline, but instead the entropy-minimization following the original work~\citep{miyato2018virtual}.
We utilized a single 24G GPU for the training.
For the ANLI, we follow the hyper-parameter suggestion from the official repository.\footnote{\url{https://github.com/facebookresearch/anli}}, where we train with the batch size of 128 and the maximum sequence length of 156.
We experimented with eight 32G GPUs for the training.

Throughout the experiments, we tune the learning rate in between \{2e-5, 3e-5\}.
For the evaluation of topic classification datasets, we use BERT-base-uncased~\citep{devlin2019bert} as a backbone model and its wordpiece~\citep{Schuster2012japkor} vocabulary as $V$.
As for the ANLI, we use RoBERTa-Large~\citep{liu2019roberta} as a backbone model and its vocabulary as $V$.
